# Supplementary material for: Dynamic Tensor Product Regression
Source: arXiv:2210.03961 source file (2026-11-25)
Supplement: Supplementary file 1 [file appendix.tex]

\Zhao{We need to write a roadmap for appendix}

\iffalse
\begin{table}[t]
    \centering
    \begin{tabular}{|l|l|l|l|} \hline
       {\bf Refs} & {\bf Initialization time} & {\bf Query time} &  {\bf Update time}\\ \hline
       Baseline Algorithm & $\tilde{O}(d (\sum_{i=1}^q \nnz(A_i) + d^3 q3^q/(\epsilon^2 \delta) + \nnz(b))$ & 3 & 4 \\ \hline
       Tree & ?? & ?? & ??  \\ \hline
    \end{tabular}
    \caption{Dynamic Kronecker Product Data Structures
    }
    \label{tab:dynamic_kronecker_data_structures}
\end{table}
\fi

\section{Baseline Algorithm}
We present a baseline algorithm for dynamic Kronecker product regression problem. 

\begin{algorithm}[]\caption{Baseline Dynamic Kronecker Regression Algorithm (using \cite{djssw19})}\label{alg:baseline_leverage_score}
\begin{algorithmic}[1]
\State {\bf data structure } ??? \Comment{Theorem~\ref{thm:baseline_leverage_score}}
\State {\bf members}
\State \hspace{4mm} $A_1, A_2, \dots, A_q$ where $A_i \in \R^{n_i \times d_i}$ for all $i \in [q]$
\State \hspace{4mm} $b \in \R^{n_1 n_2 \dots n_q}$
\State {\bf end members}
\State
\Procedure{Initialize}{$A_1 \in \R^{n_1 \times d_1}, A_2 \in \R^{n_2 \times d_2},\dots, A_q \in \R^{n_q \times d_q}, b \in \R^{n_1 n_2 \dots n_q}$}
    \State $A_1 \gets A_1, A_2 \gets A_2, \dots, A_q \gets A_q$
    \State $b \gets b$
    \State $d \gets \prod_{i=1}^q d_i$, $n \gets \prod_{i=1}^q n_i$
\EndProcedure
\State
\Procedure{Update}{$i \in [q], j \in [n_i], k \in [d_i], \Delta \in \R$}
    \State $A_i[j,k] \gets A_i[j,k] + \Delta$
\EndProcedure
\State
\Procedure{Query}{$x$}
	\State  $m \gets \Theta(d/(\delta\eps^2))$
	\State Compute approximate leverage scores $\tilde{\sigma}_i(A_j)$ for all $j \in [q],$ $i \in [n_j]$.
	\State Construct diagonal leverage score sampling matrix $D \in \R^{n \times n}$, with $m$ non-zero entries
	\State Compute (via the psuedo-inverse) \\ \hspace{30mm} $ \wh{x} = \arg \min_{x \in \R^d} \| D(A_1 \otimes A_2 \otimes \cdots \otimes A_q)x - Db\|_2 $
	\State \Return $\wh{x}$
\EndProcedure
\State {\bf end data structure}
\end{algorithmic}
\end{algorithm}

\begin{theorem}[Baseline Leverage Score]
There is an algorithm that has the following procedures:
\begin{itemize}\label{thm:baseline_leverage_score}
    \item The space storage is $O(\sum_{i = 1}^q n_id_i)$.
    \item \textsc{Initialize}($A_1 \in \R^{n_1 \times d_1}, A_2 \in \R^{n_2 \times d_2},\dots, A_q \in \R^{n_q \times d_q}, b \in \R^{n_1 n_2 \dots n_q}$): Given matrices $A_1 \in \R^{n_1 \times d_1}, A_2 \in \R^{n_2 \times d_2}, \dots, A_q \in \R^{n_q \times d_q},$ and $b \in \R^{n_1 n_2 \dots n_q}$, the data-structure pre-processes in $O(\sum_{i = 1}^q nnz(A_i) + nnz(b))$ time and uses space $O(\sum_{i = 1}^q n_id_i)$.
    \item \textsc{Query}: Query outputs an approximate solution $\hat{x}$ to the Kronecker product regression problem where $\|A\hat{x} - b\|_2 \leq (1 + \epsilon) \|Ax^* - b\|_2$ with probability at least $1 - \delta$ in time $\tilde{O}(\sum_{i = 1}^q \nnz(A_i) + (dq/(\delta \epsilon))^{O(1)})$\footnote{The exponent is at most 3.} where $x^*$ is an optimal solution to the Kronecker product regression problem i.e. $x^* = \arg \min_{x \in \R^d} \|Ax - b\|_2$.
    \item \textsc{Update}({$i \in [q], j \in [n_i], k \in [d_i], \Delta \in \R$}): Takes $O(1)$ time.
\end{itemize}
\end{theorem}
